# Supplementary material for: Resource theory of asymmetric distinguishability
Source: arXiv:1905.11629 ancillary file (2019-12-11)
Supplement: Supplementary file 1 [file SDP-duals-states.pdf]

In this supplementary document, we provide proofs of the various semi-definite programming duals that appear in our paper “Resource theory of asymmetric distinguishability.” We employ the following standard form for the primal semi-definite programs:

$$\inf_{Z \geq 0} \{ \text{Tr}[BZ] : \Phi^\dagger(Z) \geq A \}, \quad (1)$$

and the dual form is given by

$$\sup_{X \geq 0} \{ \text{Tr}[AX] : \Phi(X) \leq B \}. \quad (2)$$

If strong duality holds, these two optimizations are equal.

## 1 Normalized trace distance

The normalized trace distance is given by

$$\frac{1}{2} \|\rho - \sigma\|_1 = \sup_{\Lambda \geq 0} \{ \text{Tr}[\Lambda(\rho - \sigma)] : \Lambda \leq I \}, \quad (3)$$

so that the SDP in standard form is as in (2), with

$$A = \rho - \sigma, \quad B = I, \quad \Phi = \text{id}. \quad (4)$$

This implies that  $\Phi^\dagger = \text{id}$ . Then plugging in to (1), its dual is given by

$$\inf_{Z \geq 0} \{ \text{Tr}[Z] : Z \geq \rho - \sigma \}. \quad (5)$$

## 2 Max-relative entropy

The max-relative entropy is given by

$$D_{\max}(\rho \parallel \sigma) = \log_2 \inf \{ \lambda : \rho \leq \lambda \sigma \}. \quad (6)$$

We identify

$$B = 1, \quad A = \rho, \quad \Phi^\dagger(\lambda) = \lambda \sigma. \quad (7)$$

The adjoint of  $\Phi$  is such that

$$\text{Tr}[\Phi(X)Z] = \text{Tr}[X\Phi^\dagger(Z)]. \quad (8)$$

In this case, we have that

$$\text{Tr}[\Phi^\dagger(\lambda)X] = \lambda \text{Tr}[\sigma X], \quad (9)$$

so that  $\Phi(X) = \text{Tr}[X\sigma]$ . Thus, the dual is given by plugging in to (2):

$$D_{\max}(\rho \parallel \sigma) = \log_2 \sup_{X \geq 0} \{ \text{Tr}[X\rho] : \text{Tr}[X\sigma] \leq 1 \}. \quad (10)$$

### 3 Smooth max-relative entropy

The smooth max-relative entropy  $D_{\max}^\varepsilon(\rho\|\sigma)$  is defined as

$$D_{\max}^\varepsilon(\rho\|\sigma) := \log \inf \left\{ \lambda : \tilde{\rho} \leq \lambda\sigma, \frac{1}{2} \|\tilde{\rho} - \rho\|_1 \leq \varepsilon, \tilde{\rho} \geq 0, \text{Tr}[\tilde{\rho}] = 1 \right\}. \quad (11)$$

Using the fact that

$$\frac{1}{2} \|\tilde{\rho} - \rho\|_1 = \inf \{ \text{Tr}[Y] : Y \geq \rho - \tilde{\rho}, Y \geq 0 \}, \quad (12)$$

we can then write  $D_{\max}^\varepsilon(\rho\|\sigma)$  as the following SDP:

$$D_{\max}^\varepsilon(\rho\|\sigma) = \log \inf \left\{ \lambda : \tilde{\rho} \leq \lambda\sigma, \text{Tr}[Y] \leq \varepsilon, \tilde{\rho} \geq 0, \right. \\ \left. \text{Tr}[\tilde{\rho}] = 1, Y \geq \rho - \tilde{\rho}, Y \geq 0 \right\}. \quad (13)$$

The dual SDP is then given by

$$D_{\max}^\varepsilon(\rho\|\sigma) = \log \sup \{ \text{Tr}[Q\rho] + \mu - \varepsilon t \} \quad (14)$$

$$\begin{aligned} & \text{subject to} \\ & \text{Tr}[X\sigma] \leq 1, \\ & Q + \mu I \leq X, \\ & Q \leq tI, \\ & X, Q, t \geq 0, \mu \in \mathbb{R} \end{aligned} \quad (15)$$

To see this, consider that we can rewrite the following

$$\inf \{ \lambda : \tilde{\rho} \leq \lambda\sigma, \text{Tr}[Y] \leq \varepsilon, \text{Tr}[\tilde{\rho}] = 1, Y \geq \rho - \tilde{\rho}, \tilde{\rho}, Y, \lambda \geq 0 \} \quad (16)$$

as

$$\begin{aligned} & \inf \{ \text{Tr}[BZ] : \Phi^\dagger(Z) \geq A, Z \geq 0 \} \\ & = \sup \{ \text{Tr}[AX] : \Phi(X) \leq B, X \geq 0 \}, \end{aligned} \quad (17)$$

with

$$Z = \begin{bmatrix} \lambda & 0 & 0 \\ 0 & \tilde{\rho} & 0 \\ 0 & 0 & Y \end{bmatrix}, \quad B = \begin{bmatrix} 1 & 0 & 0 \\ 0 & 0 & 0 \\ 0 & 0 & 0 \end{bmatrix}, \quad (18)$$

$$\Phi^\dagger(Z) = \begin{bmatrix} \lambda\sigma - \tilde{\rho} & 0 & 0 & 0 & 0 \\ 0 & Y + \tilde{\rho} & 0 & 0 & 0 \\ 0 & 0 & -\text{Tr}[\tilde{\rho}] & 0 & 0 \\ 0 & 0 & 0 & \text{Tr}[\tilde{\rho}] & 0 \\ 0 & 0 & 0 & 0 & -\text{Tr}[Y] \end{bmatrix}, \quad (19)$$

$$A = \begin{bmatrix} 0 & 0 & 0 & 0 & 0 \\ 0 & \rho & 0 & 0 & 0 \\ 0 & 0 & -1 & 0 & 0 \\ 0 & 0 & 0 & 1 & 0 \\ 0 & 0 & 0 & 0 & -\varepsilon \end{bmatrix}. \quad (20)$$

So we need to compute the dual of  $\Phi^\dagger$ , which is given by

$$\text{Tr}[X\Phi^\dagger(Z)] = \text{Tr}[\Phi(X)Z], \quad (21)$$

where

$$X = \begin{bmatrix} X_1 & 0 & 0 & 0 & 0 \\ 0 & X_2 & 0 & 0 & 0 \\ 0 & 0 & \mu_1 & 0 & 0 \\ 0 & 0 & 0 & \mu_2 & 0 \\ 0 & 0 & 0 & 0 & \mu_3 \end{bmatrix}. \quad (22)$$

Then we find that

$$\text{Tr}[X\Phi^\dagger(Z)] \quad (23)$$

$$= \text{Tr}[X_1(\lambda\sigma - \tilde{\rho})] + \text{Tr}[X_2(Y + \tilde{\rho})] - \mu_1 \text{Tr}[\tilde{\rho}] + \mu_2 \text{Tr}[\tilde{\rho}] - \mu_3 \text{Tr}[Y] \quad (24)$$

$$= \lambda \text{Tr}[X_1\sigma] + \text{Tr}[\tilde{\rho}(X_2 - X_1 + (\mu_2 - \mu_1)I)] + \text{Tr}[Y(X_2 - \mu_3I)] \quad (25)$$

$$= \text{Tr} \left[ \begin{bmatrix} \lambda & 0 & 0 \\ 0 & \tilde{\rho} & 0 \\ 0 & 0 & Y \end{bmatrix} \begin{bmatrix} \text{Tr}[X_1\sigma] & 0 & 0 \\ 0 & X_2 - X_1 + (\mu_2 - \mu_1)I & 0 \\ 0 & 0 & X_2 - \mu_3I \end{bmatrix} \right]. \quad (26)$$

So then

$$\Phi \left( \begin{bmatrix} X_1 & 0 & 0 & 0 & 0 \\ 0 & X_2 & 0 & 0 & 0 \\ 0 & 0 & \mu_1 & 0 & 0 \\ 0 & 0 & 0 & \mu_2 & 0 \\ 0 & 0 & 0 & 0 & \mu_3 \end{bmatrix} \right) = \begin{bmatrix} \text{Tr}[X_1\sigma] & 0 & 0 \\ 0 & X_2 - X_1 + (\mu_2 - \mu_1)I & 0 \\ 0 & 0 & X_2 - \mu_3I \end{bmatrix}. \quad (27)$$

Then the dual is given by

$$\sup \{ \text{Tr}[AX] : \Phi(X) \leq B, X \geq 0 \} \quad (28)$$

$$= \sup \text{Tr} \left( \begin{bmatrix} 0 & 0 & 0 & 0 & 0 \\ 0 & \rho & 0 & 0 & 0 \\ 0 & 0 & -1 & 0 & 0 \\ 0 & 0 & 0 & 1 & 0 \\ 0 & 0 & 0 & 0 & -\varepsilon \end{bmatrix} \begin{bmatrix} X_1 & 0 & 0 & 0 & 0 \\ 0 & X_2 & 0 & 0 & 0 \\ 0 & 0 & \mu_1 & 0 & 0 \\ 0 & 0 & 0 & \mu_2 & 0 \\ 0 & 0 & 0 & 0 & \mu_3 \end{bmatrix} \right) \quad (29)$$

$$: \begin{bmatrix} \text{Tr}[X_1\sigma] & 0 & 0 \\ 0 & X_2 - X_1 + (\mu_2 - \mu_1)I & 0 \\ 0 & 0 & X_2 - \mu_3I \end{bmatrix} \leq \begin{bmatrix} 1 & 0 & 0 \\ 0 & 0 & 0 \\ 0 & 0 & 0 \end{bmatrix}, X \geq 0 \quad (30)$$

which can be written as

$$\sup \left\{ \begin{array}{l} \text{Tr}[X_2\rho] + \mu_2 - \mu_1 - \varepsilon\mu_3 : \\ \text{Tr}[X_1\sigma] \leq 1, \\ X_2 + (\mu_2 - \mu_1)I \leq X_1, \\ X_2 \leq \mu_3I, \\ X_1, X_2, \mu_1, \mu_2, \mu_3 \geq 0 \end{array} \right\} \quad (31)$$

$$= \sup \left\{ \begin{array}{l} \text{Tr}[X_2 \rho] + \mu - \varepsilon \mu_3 : \\ \text{Tr}[X_1 \sigma] \leq 1, \\ X_2 + \mu I \leq X_1, \\ X_2 \leq \mu_3 I, \\ X_1, X_2, \mu_3 \geq 0, \mu \in \mathbb{R} \end{array} \right\}. \quad (32)$$

$$= \sup \left\{ \begin{array}{l} \text{Tr}[Q \rho] + \mu - \varepsilon t : \\ \text{Tr}[X \sigma] \leq 1, \\ Q + \mu I \leq X, \\ Q \leq t I, \\ X, Q, t \geq 0, \mu \in \mathbb{R} \end{array} \right\} \quad (33)$$

## 4 Approximate box transformation problem

The approximate box transformation problem is given by the following semi-definite program.

$$\inf_{Y_B, J_{RB}^N} \left\{ \begin{array}{l} \text{Tr}[Y_B] : \\ Y_B + \text{Tr}_R[T_R(\rho_R)J_{RB}^N] \geq \tau_B, \\ \text{Tr}_R[T_R(\sigma_R)J_{RB}^N] = \omega_B, \\ \text{Tr}_B[J_{RB}^N] = I_R, \quad Y_B, J_{RB}^N \geq 0 \end{array} \right\} \quad (34)$$

We rewrite this in the form of (1). Consider that

$$Z = \begin{bmatrix} Y_B & 0 \\ 0 & J_{RB}^N \end{bmatrix}, \quad B = \begin{bmatrix} I_B & 0 \\ 0 & 0 \end{bmatrix}, \quad (35)$$

$$\Phi^\dagger(Z) = \text{diag} \begin{bmatrix} Y_B + \text{Tr}_R[T_R(\rho_R)J_{RB}^N] \\ \text{Tr}_R[T_R(\sigma_R)J_{RB}^N] \\ -\text{Tr}_R[T_R(\sigma_R)J_{RB}^N] \\ \text{Tr}_B[J_{RB}^N] \\ -\text{Tr}_B[J_{RB}^N] \end{bmatrix} \quad (36)$$

$$A = \begin{bmatrix} \tau_B & 0 & 0 & 0 & 0 \\ 0 & \omega_B & 0 & 0 & 0 \\ 0 & 0 & -\omega_B & 0 & 0 \\ 0 & 0 & 0 & I_R & 0 \\ 0 & 0 & 0 & 0 & -I_R \end{bmatrix}. \quad (37)$$

Our goal is then to compute the adjoint of  $\Phi^\dagger$  by using

$$\text{Tr}[X \Phi^\dagger(Z)] = \text{Tr}[\Phi(X)Z], \quad (38)$$

with

$$X = \begin{bmatrix} X_B^1 & 0 & 0 & 0 & 0 \\ 0 & X_B^2 & 0 & 0 & 0 \\ 0 & 0 & X_B^3 & 0 & 0 \\ 0 & 0 & 0 & X_R^4 & 0 \\ 0 & 0 & 0 & 0 & X_R^5 \end{bmatrix} \quad (39)$$

This implies that

$$\text{Tr}[X\Phi^\dagger(Z)] \quad (40)$$

$$= \text{Tr}[X_B^1 (Y_B + \text{Tr}_R[\rho_R] J_{RB}^\mathcal{N})] + \text{Tr}[X_B^2 (\text{Tr}_R[\sigma_R] J_{RB}^\mathcal{N})] \quad (41)$$

$$- \text{Tr}[X_B^3 (\text{Tr}_R[\sigma_R] J_{RB}^\mathcal{N})] + \text{Tr}[X_R^4 (\text{Tr}_B[J_{RB}^\mathcal{N}])] - \text{Tr}[X_R^5 (\text{Tr}_B[J_{RB}^\mathcal{N}])] \quad (42)$$

$$= \text{Tr}[Y_B X_B^1] + \text{Tr}[(T_R(\rho_R) \otimes X_B^1) J_{RB}^\mathcal{N}] + \text{Tr}[(T_R(\sigma_R) \otimes X_B^2) J_{RB}^\mathcal{N}] \quad (43)$$

$$- \text{Tr}[(T_R(\sigma_R) \otimes X_B^3) J_{RB}^\mathcal{N}] + \text{Tr}[(X_R^4 \otimes I_B) J_{RB}^\mathcal{N}] - \text{Tr}[(X_R^5 \otimes I_B) J_{RB}^\mathcal{N}] \quad (44)$$

$$= \text{Tr}[Y_B X_B^1] + \quad (45)$$

$$\text{Tr}[(T_R(\rho_R) \otimes X_B^1 + T_R(\sigma_R) \otimes (X_B^2 - X_B^3) + (X_R^4 - X_R^5) \otimes I_B) J_{RB}^\mathcal{N}]. \quad (46)$$

So then

$$\Phi(X) = \begin{bmatrix} X_B^1 & 0 \\ 0 & (T_R(\rho_R) \otimes X_B^1 + T_R(\sigma_R) \otimes (X_B^2 - X_B^3) + (X_R^4 - X_R^5) \otimes I_B) \end{bmatrix}. \quad (47)$$

This finally implies that the dual is given by

$$\sup_X \left\{ \begin{array}{c} \text{Tr} \left[ \text{diag} \begin{bmatrix} \tau_B \\ \omega_B \\ -\omega_B \\ I_R \\ -I_R \end{bmatrix} \text{diag} \begin{bmatrix} X_B^1 \\ X_B^2 \\ X_B^3 \\ X_R^4 \\ X_R^5 \end{bmatrix} \right] : \\ X_B^1, X_B^2, X_B^3, X_R^4, X_R^5 \geq 0, \\ \begin{bmatrix} X_B^1 & 0 \\ 0 & (T_R(\rho_R) \otimes X_B^1 + T_R(\sigma_R) \otimes (X_B^2 - X_B^3) + (X_R^4 - X_R^5) \otimes I_B) \end{bmatrix} \\ \leq \begin{bmatrix} I_B & 0 \\ 0 & 0 \end{bmatrix} \end{array} \right\} \quad (48)$$

$$= \sup_X \left\{ \begin{array}{c} \text{Tr}[\tau_B X_B^1] + \text{Tr}[\omega_B (X_B^2 - X_B^3)] + \text{Tr}[X_R^4 - X_R^5] : \\ X_B^1 \leq I_B, \\ (T_R(\rho_R) \otimes X_B^1 + T_R(\sigma_R) \otimes (X_B^2 - X_B^3) + (X_R^4 - X_R^5) \otimes I_B) \leq 0, \\ X_B^1, X_B^2, X_B^3, X_R^4, X_R^5 \geq 0, \end{array} \right\} \quad (49)$$

$$= \sup_{X_B, W_B, Z_R} \left\{ \begin{array}{c} \text{Tr}[\tau_B X_B] + \text{Tr}[\omega_B W_B] + \text{Tr}[Z_R] : \\ X_B \leq I_B, \\ T_R(\rho_R) \otimes X_B + T_R(\sigma_R) \otimes W_B + Z_R \otimes I_B \leq 0, \\ X_B \geq 0, W_B, Z_R \in \text{Herm} \end{array} \right\} \quad (50)$$
